# Supplementary material for: Token-Level Fuzzing
Source: arXiv:2304.02103 source file (2023-04-04)
Supplement: Supplementary file 1 [file appendix.tex]

\section{Major Revision Changes}
\label{sec:major}

We thank the reviewers for their valuable feedback. In the following paragraphs, we list each of the requested items for the major revision and comment on how we addressed them. We also made numerous other edits to the paper to add more details and clean up the presentation.

\subsection{Evaluation against newer Fuzzing tools to demonstrate effectiveness}

One request was for us to include one additional JavaScript fuzzer into our experimental evaluation. We decided to select Superion, both because it was one of the recommendations from the reviewers, but also because we believe that it is a good representative of tools that leverage grammar-based evolutionary fuzzing (on ASTs).

In our results (shown in Section 5), we find that Superion only outperformed AFL by a bit, while the other fuzzers and \toolname{} found more bugs and achieved higher coverage. We worked hard to ensure that we compare against the state-of-the-art, and we hope our results show that the tools that we selected for our comparative evaluation are indeed some of the best publicly available JavaScript fuzzers.

\subsection{Detailed statistical evaluation analysis including break down of the identified bugs.}

As requested, we included a table (Table 4 in Section 5) that identifies which bugs were found by which fuzzer. We can see that most of the bugs found by \toolname{} do not overlap with bugs found by other tools, supporting a key claim that Token-Level Fuzzing is able to detect bugs that other fuzzing approaches will miss.

We also performed a statistical evaluation, providing confidence intervals for the number of bugs found in each run. The confidence intervals are shown in Table 2 (Section 5).

\subsection{Extend the evaluation by at least one recent fuzzer that has been tested on JavaScript}

As mentioned previously, we added Superion to the evaluation for this major revision.

\subsection{Either provide p-values or 95\%-confidence-intervals for the number of bugs found}

We added confidence intervals around the average number of bugs found by each fuzzer. The information can be found in Table 2. As can be seen from the table, our statistical analysis strengthens the claim that Token-Level Fuzzing consistently delivers strong results, and our numbers are not the result of luck or a statistical fluke.

\subsection{Provide an overview that shows which bug has been found by which fuzzer.}

As requested, we included a table showing this information (in Table 4). Our data shows that most of the bugs found by our tool were not found by other tools.

\subsection{ Increase the number of trials to at least 5 to improve the statistical significance}

The reviewers asked us to increase the number of runs from 3 to 5 for all of the fuzzers and  JavaScript targets. We did so and include updated numbers as well as graphsin the paper. Interestingly, adding more runs resulted in a slight increase in the number of bugs found by  \toolname{} and by CodeAlchemist. We hope this shows a higher statistical significance of the results from our experiments.

\subsection{Extend the related work section to include the work of Park et al}

The reviewers asked us to expand on the work by Park et al. on "Aspect Preserving Mutations" and to include related work on fuzzers that mutate on a grammar-level (bridging the gap between grammar-based and evolutionary fuzzers). We extended our discussion of Park's work in Section 2.2.2 and added references to (and discussion of) Montage [27] and Nautilus [1].

\subsection{When comparing the total number of bugs found, mention that testing on the latest version may introduce a bias}

We acknowledge that there could be a potential bias due to the fact that the bugs that other tools had found were already patched in the versions of the JavaScript engines that we analyzed. We added appropriate language to make readers aware of this issue and clarify that the lack of bugs found by other tools does not directly indicate a lack of performance. We wrote about this issue in two places: Once at the start of the evaluation section (towards the end of Section 5.1) and then at the end of Section 5.3 (that covers the comparison with the four other tools).
